# Supplementary material for: M6: A Chinese Multimodal Pretrainer
Source: arXiv:2103.00823 source file (2021-05-29)
Supplement: Supplementary file 1 [file 6.appendix.tex]

\section{Appendix}
%You may include other additional sections here.

\begin{table*}
  \centering
  \small
  \caption{Summarization of implemented models for node classification and graph classification tasks.}
  \begin{tabular}{c|c|l|c}
  \toprule
  Task & \multicolumn{2}{c|}{\textit{Characteristics}} & Models \\
  \midrule
  \multirow{4}{*}{\makecell{Node Classification \\ (Unsupervised)}} & 
  \multirow{2}{*}{\textit{Matrix Factorization}} & &
  SpectralClustering~\cite{tang2011leveraging} \\
  \cmidrule{3-4}
  & & \textit{With high-order neighborhood} & NetMF~\cite{qiu2018network}, ProNE~\cite{zhang2019prone}, NetSMF~\cite{qiu2019netsmf}, HOPE~\cite{ou2016asymmetric}, GraRep~\cite{cao2015grarep}\\
  \cmidrule{2-4}
  & \multirow{2}{*}{\textit{Skip-gram}} &
  & LINE~\cite{tang2015line} \\
  \cmidrule{3-4}
  & & \textit{With high-order neighborhood} & 
  DeepWalk~\cite{perozzi2014deepwalk}, Node2vec~\cite{grover2016node2vec} \\
  \midrule
  
  \multirow{4}{*}{\makecell{Node Classification \\(with GNN)}} & 
  \multirow{3}{*}{\textit{Semi-supervised}} &
   \textit{} & 
  GCN~\cite{kipf2016semi}, GAT~\cite{Velickovic:18GAT}, JK-Net~\cite{xu2018representation}, ChebyNet~\cite{defferrard2016chebynet}, GCNII~\cite{chen2020gcnii} \\
  \cmidrule{3-4}
  & & \textit{With random propagation} & DropEdge~\cite{rong2019dropedge}, Graph-Unet~\cite{gao2019graph}, GraphSAINT~\cite{graphsaint-iclr20}, GRAND~\cite{feng2020grand} \\
  \cmidrule{3-4}
  & & \textit{With diffusion} & GDC~\cite{klicpera2019diffusion}, APPNP~\cite{klicpera2019appnp}, GRAND~\cite{feng2020grand}, PPRGo~\cite{bojchevski2020scaling} \\
  \cmidrule{2-4} 
  & \textit{Self-supervisd} & \textit{Contrastive methods} & MVGRL~\cite{hassani2020mvgrl}, DGI~\cite{velickovic2019dgi} \\
  \midrule

  \multirow{5}{*}{Graph Classification} & 
  \multirow{3}{*}{\textit{Supervisd}} &
  \textit{CNN method} &
  PATCHY\_SAN~\cite{niepert2016patchy} \\
  \cmidrule{3-4}
  & & \textit{Global pooling} & GIN~\cite{xu2019gin}, SortPool~\cite{zhang2018sortpool}, DGCNN~\cite{wang2019dgcnn} \\
  \cmidrule{3-4}
  & & \textit{Hierachical pooling} & DiffPool~\cite{ying2018diffpool}, SAGPool~\cite{lee2019sagpool} \\
  \cmidrule{2-4}
  & \multirow{2}{*}{\textit{Unsupervised}} & 
  \textit{Kernel methods} &
  DGK~\cite{yanardag2015dgk}, graph2vec~\cite{narayanan2017graph2vec} \\
  \cmidrule{3-4}
  & & \textit{GNN method} & Infograph~\cite{sun2019infograph} \\
  \bottomrule
  \end{tabular}
  \label{tab:summary_models}
  \normalsize
\end{table*}

\hide{
\begin{table}[htbp]
    \caption{Dataset statistics for heterogeneous node classification}
	\begin{tabular}{l|r|r|r|c}
		\toprule
		Dataset & \#Nodes & \#Edges & \#Features & \#Classes\\
		\midrule
		DBLP & 18,405 & 67,946 & 334 & 4 \\
		ACM & 8,994 & 25,922 & 1,902 & 3 \\
		IMDB & 12,772 & 37,288 & 1,256 & 3 \\
		\bottomrule
	\end{tabular}
	\label{hnc_dataset}
\end{table}

\begin{table}[htbp]
    \caption{Dataset statistics for multiplex heterogeneous link prediction}
	\begin{tabular}{lrrcc}
		\toprule
		Dataset  & \#Nodes    & \#Edges & \#n-types & \#e-types \\ 
		\midrule
		Amazon & 10,166 & 148,865 & 1 & 2 \\
		YouTube & 2,000 & 1,310,617 & 1 & 5 \\
		Twitter & 10,000 & 331,899 & 1 & 4 \\
		\bottomrule
	\end{tabular}
	\label{mlp_dataset}
\end{table}

\subsection{Datasets}
% dataset source (link)

\vpara{Heterogeneous Node Classification}
Table~\ref{hnc_dataset} shows the dataset statistics used in CogDL for the heterogeneous node classification. 

\vpara{Multiplex Link Prediction.}
Three multiplex datasets, including Amazon, YouTube, and Twitter, are used in our CogDL. 
Table~\ref{mlp_dataset} shows the dataset statistics used in CogDL for the multiplex link prediction. 
Amazon is a dataset of product reviews and metadata from Amazon. 
YouTube is a multi-dimensional bidirectional network dataset consists of 5 types of interactions (edges) between YouTube users. 
Twitter is a dataset about tweets posted on Twitter about the discovery of the Higgs boson between 1st and 7th, July 2012. It is made up of 4 directional relationships between Twitter users.

\vpara{Knowledge Graph Completion.}
FB15k-238, WN18, and WN18RR.
}

\subsection{Models}
\label{appendix:models}
In this section, we list the details of all models implemented in CogDL. % for unsupervised node classification, semi-supervised node classification, and graph classification.
We summarize these models in Table~\ref{tab:summary_models}.

\vpara{Unsupervised Node Classification}

\begin{itemize}[leftmargin=*]
    \item SpectralClustering~\cite{tang2011leveraging} generates node representations from the $d$-smallest eigenvectors of the normalized graph Laplacian.
	\item DeepWalk~\cite{perozzi2014deepwalk} transforms a graph structure into linear sequences by truncating random walks and processing the sequences using Skip-gram with hierarchical softmax. 
	\item LINE~\cite{tang2015line} defines loss functions to preserve first-order or second-order proximity separately and concatenates two representations together. 
	\item node2vec~\cite{grover2016node2vec} designs a biased random walk procedure with Breadth-first Sampling (BFS) and Depth-first Sampling (DFS) to make a trade off between homophily similarity and structural equivalence similarity.
	\item GraRep~\cite{cao2015grarep} decomposes $k$-step probability transition matrix to train the node embedding, then concatenate all $k$-step representations.
	\item HOPE~\cite{ou2016asymmetric} approximates high-order proximity based on factorizing the Katz matrix.
% 	\item SDNE~\cite{wang2016structural} utilizes a deep model with non-linear functions to exploit the first-order and second-order proximity jointly to preserve the network structure.
	\item NetMF~\cite{qiu2018network} shows that Skip-gram models with negative sampling like Deepwalk, LINE can be unified into the matrix factorization framework with closed forms.
	\item ProNE~\cite{zhang2019prone}  firstly transforms the graph representation learning into decomposition of a sparse matrix, and further improves the performance through spectral propagation technology.
	\item NetSMF ~\cite{qiu2019netsmf} addresses the efficiency and scalability challenges faced by the NetMF model via achieving a sparsification of the (dense) NetMF matrix.
\end{itemize}

\vpara{Semi-supervised Node Classification}

\begin{itemize}[leftmargin=*]
	\item Chebyshev~\cite{defferrard2016chebynet} presents a formulation of CNNs in the context of spectral graph theory, which provides the necessary mathematical background and efficient numerical schemes to design fast localized convolutional filters on graphs.
	\item GCN~\cite{kipf2016semi} proposes a well-behaved layer-wise propagation rule for neural network models which operate directly on graphs and are motivated from a first-order approximation of spectral graph convolutions.
	\item GAT~\cite{Velickovic:18GAT} presents graph attention networks (GATs), a novel convolution-style neural networks that operate on graph-structured data, leveraging masked self-attentional layers.
	\item GraphSAGE~\cite{hamilton2017inductive} introduces a novel approach that allows embeddings to be efficiently generated for unseen nodes by aggregating feature information from a node's local neighborhood.
	\item APPNP~\cite{klicpera2019appnp} derives a propagation scheme from personalized PageRank by adding initial residual connection to balance locality and leverage information from a large neighborhood.
	\item DGI~\cite{velickovic2019dgi} indtroduces an approach to maximize mutual information between local representation and corresponding summaries of graphs to learn node representation in an unsupervised manner.
	\item GCNII~\cite{chen2020gcnii} extends GCN to a deep model by using identity mapping and initial residual connection to resolve over-smoothing. 
	\item MVGRL~\cite{hassani2020mvgrl} proposes to use graph diffusion for data augmentation and contrasts structural views of graphs for self-supervised learning. MVGRL also maximizes local-global mutual information.
	\item GRAND~\cite{feng2020grand} proposes to combine random propagation and consistency regularization to optimize the prediction consistency of unlabeled data across different data augmentations.
	\item DropEdge~\cite{rong2019dropedge} randomly removes a certain number of edges from the input graph at each training epoch, acting like a data augmenter and also a message-passing reducer to alleviate over-fitting and over-smoothing issues.
	\item Graph-Unet~\cite{gao2019graph} uses novel graph pooling (gPool) and unpooling (gUnpool) operations where gPool adaptively selects some nodes to form a smaller graph based on their scalar projection values on a trainable projection vector and gUnpool restores the graph.
	\item GDC~\cite{klicpera2019diffusion} leverages generalized graph diffusion, such as heat kernel and personalized PageRank, to alleviate the problem of noisy and often arbitrarily defined edges in real graphs.
	\item PPRGo~\cite{bojchevski2020scaling} utilizes an efficient approximation of information diffusion in GNNs based on personalized PageRank, resulting in significant speed gains.
	\item GraphSAINT~\cite{graphsaint-iclr20} constructs minibatches by sampling the training graph and trains a full GCN on sampled subgraphs. 
\end{itemize}

\vpara{Graph Classification}

\begin{itemize}[leftmargin=*]
    \item GIN~\cite{xu2019gin} presents graph isomorphism network, which adjusts the weight of the central node with learning and aims to make GNN as powerful as the WeisfeilerLehman graph isomorphism test.
    \item DiffPool~\cite{ying2018diffpool} proposes a differentiable pooling and generates hierachical representation of graphs. It learns a cluster assignment matrix and can be implemented based on any GNN.
    \item SAGPool~\cite{lee2019sagpool} proposes a hierachical graph pooling method based on self-attention and considers both node features and graph topology.
    \item SortPool~\cite{zhang2018sortpool} rearanges nodes by sorting them according to their structural roles within the graph and then perform pooling on these nodes. Node features derived from graph convolutions are used as continuous WL colors for sorting nodes.
    \item PATCHY\_SAN~\cite{niepert2016patchy} orders neighbors of each node according to their graph labelings and selects the top $q$ neighbors. The graph labelings are derived by degree, centrality and other node scores.
    \item DGCNN~\cite{wang2019dgcnn} builds a subgraph for each node with KNN based on node features and then applies graph convolution to the reconstructed graph.
    \item Infograph~\cite{sun2019infograph} applies contrastive learning to graph learning by maximizing the mutual information between both graph-level representation and node-level representation in an unsupervised manner.
    \item graph2vec~\cite{narayanan2017graph2vec} follows skip-gram's training process and considers the set of all rooted subgraphs around each node as its vocabulary.
    \item Deep Graph Kernels (DGK)~\cite{yanardag2015dgk} learns latent representation for subgraph structures based on graph kernels in graphs with Skip-gram method. 
\end{itemize}

\subsection{CogDL Package}

In this section, we introduce the key components of the CogDL package, including \textit{Task}, \textit{Dataset}, \textit{Model}, and \textit{Trainer}. 
% The key point is to first build a task through arguments $task = build\_task(args)$ and then run $ret=task.train()$ to train models on given datasets and return the performance.
% We also provide a more easy-to-use usage for experiments through $experiment$ API. The details of the usage can be found in the Appendix~\ref{app:cogdl-usage}.

% ------ Task ------------
\subsubsection{Task}
The model and dataset are specified in \textit{args} and built in \textit{task}. \textit{train} is the only exposed API for a task and integrates the training and evaluation. Flexiblely, loss optimization can also be implemented in \textit{train} for task-specific targets. \textit{task.train()} runs the training and evaluation of models and datasets specified in \textit{args} and returns the performance. After the training, parameters of model and node/graph representations will be saved for further plan.

% ------ Dataset ------------
\subsubsection{Dataset}
The \textit{Dataset} component reads in data from a persistent storage and processes the graph to produce tensors of the appropriate types. 
The library provides two ways to fit a customized dataset. One way is to convert raw data files into the required format in CogDL and specify the argument $data\_path$, then CogDL will read and process the data with pre-defined functions. In addition, the library allows developers to define customized dataset class. 
%As shown in the following code snippet, the user reads in, processes and caches the data with overrided \textit{process} function. 
The loss function and metric evaluator should be set. Finally the customized dataset must be "registered" to CogDL.

\noindent
\begin{lstlisting}[language=Python,breaklines=True,frame=single]
@register_dataset("my_dataset")
class MyDataset(BaseDataset):
  ...
  def get_evaluator(self):
    return accuracy
  def get_loss_fn(self):
    return cross_entropy_loss
\end{lstlisting}

% ------ Model ------------
\subsubsection{Model}\label{subsection:model}
A \textit{Model} in the library comprises of \textit{model builder}, \textit{forward propagation} and \textit{loss calculation}. APIs described below are implemented in each model to provide an unified paradigm for usage. \textit{add\_args} and \textit{build\_model\_from\_args} are used to build up a model with model-specific hyper-parameters. \textit{loss} takes in the data, calls the core \textit{forward} function and returns the loss in one propagation. The loss can consist of auxiliary parts for training, like regularization loss. In addition, the library supports specifies a customized trainer for a model. Each model should be \textit{registered} in the library. The code snippet below shows a simple implementation of a GNN model.

\noindent
\begin{lstlisting}[language=Python,breaklines=True,frame=single]
@register("sslgnn")
class SSLGNNModel(nn.Module):
  def add_args(parser):
    parser.add_argument("--wd", type=float,)
  
  def loss(self, data):
    pred = self.forward(x, edge_index)
    return loss_fn(pred, labels) + self.wd * norm(pred)/2
  
  def get_trainer():
    return SelfSupervisedTrainer
\end{lstlisting}

% ----- Trainer ------------
\subsubsection{Trainer}
\label{pkg:trainer}
\textit{Trainer} is a supplement component for \textit{Task}. The training or evaluation of some models are special and incompatible with the general paradigm in CogDL. In such cases, a custom-built trainer can be constructed in CogDL and specified in the model with $get\_trainer$, as show in Section ~\ref{subsection:model}. \textit{trainer.fit} , which is similar to the function \textit{task.train} and covers training and evaluation, takes model and dataset as input and returns the performance.
\textit{Trainer} is used only when it is specified in a model, and then the trainer will take over the process. The code snippet below together with the snippet in Section ~\ref{subsection:model} shows how a trainer is specified and used.

\noindent
\begin{lstlisting}[language=Python,breaklines=True,frame=single]
class SelfSupervisedTrainer(BaseTrainer):
  def fit(self, model, dataset):
    """Training Process."""

class NodeClassification(BaseTask):
  def __init__(self, args):
    ...
    self.trainer = self.model.get_trainer()

  def train(self):
    if self.trainer is not None:
      result = self.trainer.fit(self.model, self.dataset)
\end{lstlisting}

% \subsubsection{An example of func\_search}
% \label{pkg:func_search}
% \noindent
% \begin{lstlisting}[language=Python,breaklines=true,frame=single]
% def func_search(trial):
%     return {
%         "lr": trial.suggest_categorical("lr", [1e-4, 1e-3, 1e-2]),
%         "dropout": trial.suggest_uniform("dropout", 0.1, 0.5),
%     }
% \end{lstlisting}

\hide{
\subsection{CogDL Usage}
\label{app:cogdl-usage}

\vpara{API Usage}
You can run all kinds of experiments through CogDL APIs, especially \textit{experiment}. You can also use your own datasets and models for experiments. 
A quickstart example is listed in the following.

\noindent
\begin{lstlisting}[language=Python,breaklines=true,frame=single]
from cogdl import experiment

# basic usage
experiment(task="node_classification", dataset="cora", model="gcn")

# set other hyper-parameters
experiment(task="node_classification", dataset="cora", model="gcn", hidden_size=32, max_epoch=200)

# run over multiple models on different seeds
experiment(task="node_classification", dataset="cora", model=["gcn", "gat"], seed=[1, 2])
\end{lstlisting}

CogDL also provide AutoML usage and allows users to easily search the hyper-parameters.

\noindent
\begin{lstlisting}[language=Python,breaklines=true,frame=single]
from cogdl import experiment

# automl usage
def func_search(trial):
    return {
        "lr": trial.suggest_categorical("lr", [1e-3, 5e-3, 1e-2]),
        "hidden_size": trial.suggest_categorical("hidden_size", [32, 64, 128]),
        "dropout": trial.suggest_uniform("dropout", 0.5, 0.8),
    }

experiment(task="node_classification", dataset="cora", model="gcn", seed=[1, 2], func_search=func_search)
\end{lstlisting}
}
\hide{
Some interesting applications can be used through pipeline API. An example is listed as follows.

\noindent
\begin{lstlisting}[language=Python,breaklines=true,frame=single]
from cogdl import pipeline

# print the statistics of datasets
stats = pipeline("dataset-stats")
stats(["cora", "citeseer"])

# visualize k-hop neighbors of seed in the dataset
visual = pipeline("dataset-visual")
visual("cora", seed=0, depth=3)

# load OAGBert model and perform inference
oagbert = pipeline("oagbert")
outputs = oagbert(["CogDL is developed by KEG, Tsinghua."])
\end{lstlisting}
}

\hide{
\vpara{Command-Line Usage.} You can use \textit{python script/train.py -{}-task task -{}-dataset dataset -{}-model model} to run models on datasets and evaluate it via the specific task. 
% For specific hyper-parameters for each model, you can find in our repository\footnote{\url{https://github.com/THUDM/cogdl/blob/master/cogdl/configs.py}}.

\begin{itemize}
	\item -{}-task. Evaluating model performances on downstream tasks like \textit{node\_classification}, \textit{unsupervised\_node\_classification}, \textit{graph\_classification}.
	\item -{}-dataset. Supported datasets include \textit{cora}, \textit{citeseer}, \textit{pumbed}, \textit{ppi}, \textit{wikipedia}, \textit{blogcatalog}, and so on.
	\item -{}-model. Supported models include \textit{gcn}, \textit{gat}, \textit{graphsage}, \textit{deepwalk}, \textit{line}, \textit{node2vec}, \textit{netmf}, \textit{netsmf}, \textit{prone}, and so on.
\end{itemize}

% \vpara{Hyper-parameters.}
We put all the hyper-parameters for reproducibility in the \textit{config} file~\footnote{\url{https://github.com/THUDM/cogdl/blob/master/cogdl/configs.py}}.
Users can easily set \textit{use\_best\_config=True} in the \textit{experiment} API or \textit{-{}-use\_best\_config} in the command-line to train the model using the best parameters in the configuration file. 
}
